# Supplementary material for: Capturing vertical information in radially symmetric flow using hyperbolic shallow water moment equations
Source: arXiv:2302.07952 source file (2025-04-02)
Supplement: Supplementary file 1 [file Appendix.tex]

\section{Appendix}

\begin{theorem}
The Jacobian of the source term \(S(U)^{(N,N)}\) of the \((N,N)\)th order Cartesian system is given by
\begin{equation*}
    S_U^{(N,N)}(U)=
    \frac{\nu}{h\lambda}
    \begin{pmatrix}
         & & & & & & \\[5pt]
         a_{0} & b_{0,0} & b_{0,1} & \cdots & b_{0,N_x} & & & \\[5pt]
         a_{1} & b_{1,0} & b_{1,1} & \cdots & b_{1,N_x} & & & \\[5pt]
         \vdots & \vdots & \vdots & \ddots & \vdots & & & \\[5pt]
         a_{N_x} & b_{N_x,0} & b_{N_x,1} & \cdots & b_{N_x,N_x} & & & \\[5pt]
         \Tilde{a}_0 & & & & & \Tilde{b}_{0,0} & \Tilde{b}_{0,1} & \cdots & \Tilde{b}_{0,N_y} \\[5pt]
         \Tilde{a}_1 & & & & & \Tilde{b}_{1,0} & \Tilde{b}_{1,1} & \cdots & \Tilde{b}_{1,N_y} \\[5pt]
         \vdots & & & & & \vdots & \vdots & \ddots & \vdots \\[5pt]
         \Tilde{a}_{N_y} & & & & & \Tilde{b}_{N_y,0} & \Tilde{b}_{N_y,1} & \cdots & \Tilde{b}_{N_y,N_y}
    \end{pmatrix},
\end{equation*}
with
\footnotesize
\begin{align*}
    &a_i = (2i+1)\left( u_m + \sum_{j=1}^{N_x} \alpha_j\left( 1+\frac{2\lambda}{h}C_{ij} \right) \right), \qquad \Tilde{a}_i= (2i+1)\left( u_m + \sum_{j=1}^{N_y} \gamma_j\left( 1+\frac{2\lambda}{h}C_{ij} \right) \right), \\[5pt]
    &b_{i,j} = -(2i+1)\left( 1+\frac{\lambda}{h}C_{ij}\right), \qquad \Tilde{b}_{i,j} = -(2i+1)\left( 1+\frac{\lambda}{h} C_{ij} \right),
\end{align*}

\normalsize
and where all other entries are zero.
\end{theorem}

\begin{proof}
We will construct the Jacobian by explicitly computing the partial derivatives.
\begin{enumerate}

    \item{\textbf{Source term corresponding to equation for \(\boldsymbol{h}\)}.} 
    
    Since the first row of the source term vector is zero, the first row of the Jacobian of the source term vector will also be zero.
    
    \item{\textbf{Derivatives of \(\boldsymbol{S_i}\), \(\boldsymbol{i=0,\cdots,N_x}\)}.}
    
    Recall that
    \begin{equation*}
        S_i=-(2i+1)\frac{\nu}{\lambda}\left( u_m+\sum_{j=1}^{N_x}\alpha_j\left( 1+\frac{\lambda}{h}C_{ij} \right) \right), \qquad i=0,\ldots,N_x.
    \end{equation*}
    A direct calculation yields
    
    \begin{align*}
        &\frac{\partial S_i}{\partial h}=(2i+1)\frac{\nu}{\lambda h} \left(u_m+\sum_{j=1}^{N_x}\alpha_j\left(1+\frac{2\lambda}{h}C_{ij}\right) \right),\\[6pt]
        &\frac{\partial S_i}{\partial (hu_m)}=-(2i+1)\frac{\nu}{\lambda h},\\[6pt]
        &\frac{\partial S_i}{\partial (h\alpha_l)}=-(2i+1)\frac{\nu}{\lambda h}\left( 1+\frac{\lambda}{h}C_{il} \right),\qquad l=1,\ldots,N_x,\\[6pt]
        &\frac{\partial S_i}{\partial (hv_m)}=0,\\[6pt]
        &\frac{\partial S_i}{\partial (h\gamma_l)}=0,\qquad l=1,\ldots,N_y,
    \end{align*}
    
    for \(i=1,\ldots,N_x\).
    
    \item{\textbf{Derivatives of \(\boldsymbol{\Tilde{S}_i}\)}, \(\boldsymbol{i=0,\ldots,N_y}\).}
    
    Recall that
    \begin{equation*}
        \Tilde{S}_i=-(2i+1)\frac{\nu}{\lambda}\left( v_m+\sum_{j=1}^{N_x}\gamma_j\left( 1+\frac{\lambda}{h}C_{ij} \right) \right), \qquad i=0,\ldots,N_y.
    \end{equation*}
    A direct calculation yields
    
    \begin{align*}
        &\frac{\partial \Tilde{S}_i}{\partial h}=(2i+1)\frac{\nu}{\lambda h} \left(v_m+\sum_{j=1}^{N_x}\gamma_j\left(1+\frac{2\lambda}{h}C_{ij}\right) \right),\\[6pt]
        &\frac{\partial \Tilde{S}_i}{\partial (hu_m)}=0,\\[6pt]
        &\frac{\partial \Tilde{S}_i}{\partial (h\alpha_l)}=0,\qquad l=1,\ldots,N_x,\\[6pt]
        &\frac{\partial \Tilde{S}_i}{\partial (hv_m)}=-(2i+1)\frac{\nu}{\lambda h},\\[6pt]
        &\frac{\partial \Tilde{S}_i}{\partial (h\gamma_l)}=-(2i+1)\frac{\nu}{\lambda h}\left( 1+\frac{\lambda}{h}C_{il} \right),\qquad l=1,\ldots,N_y.
    \end{align*}
\end{enumerate}
This completes the construction of the Jacobian.
\end{proof}
